# Supplementary material for: Hierarchical Clustering: $O(1)$-Approximation for Well-Clustered Graphs
Source: arXiv:2112.09055 source file (2021-12-16)
Supplement: Supplementary file 1 [file Appendix.tex]

% \newpage
\appendix
